# Supplementary material for: Atomicity and Factorization of Puiseux Monoids
Source: arXiv:2006.09173 source file (2020-06-13)
Supplement: Supplementary file 1 [file TwoOrMoreAppendices.tex]

% The Editorial Office Requirements for the Table of Contents cause a significant problem
%in Latex if there is only one Appendix. The Appendix is no longer labeled "A" in the TOC
%but has the word "APPENDIX" placed in front of the title of the Appendix. This can be done
%without issue IF nothing needs to be numbered by LaTeX in the Appendix. Unfortunately, most of the time
%something needs to be numbered in that single Appendix. For this reason we have included the IFTHENELSE switch
%found in this document and at the beginning of AppendixA. We assume that if you have any appendices, that you have more than one. However, you DO only have one appendix DO NOT USE THIS FILE!!!!!!!!!!!!!!!!!!!!!!!
%
% OneSingleAppendix.tex has all the settings needed to adjust for a single appendix
% you will have a major problem with your TOC if you use this file with a single appendix!!!!!

%
% Comment (or delete) all of the \input{AppendixB} commands except those you are using.
%Then open the AppendixA.tex file and continue there.

%you can add/substract individual appendices through by using the /include{appendix'X'}
% and creating/deleting the appropriate files
\appendix %
%\clearpage%

\addtocontents{toc}{\protect\addvspace{10pt}\noindent{APPENDIX} \protect\hfill\par}{}
\setcounter{equation}{0}

% % % % % % % If you have a single appendix, you should be using OneSingleAppendix.tex
% % % % % % % NOT this file

\chapter{APPENDIX}

\lipsum[1]
